# Supplementary material for: Disco4D: Disentangled 4D Human Generation and Animation from a Single Image
Source: arXiv:2409.17280 source file (2024-09-25)
Supplement: Supplementary file 1 [file animation_appendix.tex]

\begin{figure*}[hbt!]
    \centering
    % \subfigure{
    % \vspace{40pt}
    \includegraphics[width=0.95\linewidth ,keepaspectratio]{Figures/Image/anim3.pdf}
    % \rule{10cm}{3cm} % This creates a black rectangle of 6cm x 3cm
    % \rule{10cm}{3cm} % This creates a black rectangle of 6cm x 3cm
    % \vspace{-10pt}
    \caption{\small \textbf{More examples of animation results compared to Dreamgaussian4D.}}
    \label{figure:animation_appendix}
\end{figure*}
