# Supplementary material for: Disco4D: Disentangled 4D Human Generation and Animation from a Single Image
Source: arXiv:2409.17280 source file (2024-09-25)
Supplement: Supplementary file 2 [file 07_appendix.tex]

\section{Appendix}

\subsection{Preliminary}
\label{section:preliminary_extras}

\textbf{3D Gaussian Splatting} employs explicit 3D Gaussian points as its primary rendering entities. A 3D Gaussian point is mathematically defined as a function $G(x)$ denoted by
\[
G(x) = e^{-\frac{1}{2}(x-\mu)^T \Sigma^{-1} (x-\mu)},
\]
where $\mu$ and $\Sigma$ denote the spatial mean and covariance matrix, respectively. Each Gaussian is also associated with an opacity $\alpha$ and a view-dependent color $c$ represented by spherical harmonic coefficients $f$. During the rendering process from a specific viewpoint, 3D Gaussians are projected onto the view plane by splatting. The means of these 2D Gaussians are determined using the projection matrix, while the 2D covariance matrices are approximated as
$
\Sigma' = J_g W_g \Sigma W_g^T J_g^T,
$
where $W_g$ and $J_g$ denote the viewing transformation and the Jacobian of the affine approximation of the perspective projection transformation of Gaussian points. To obtain the pixel color, alpha-blending is performed on $N$ sequentially layered 2D Gaussians, starting from the front and moving toward the back. 
$
C = \sum_{i \in N} T_i \alpha_i c_i,
$
with
$
T_i = \prod_{j=1}^i (1 - \alpha_j).
$

In the splatting process, the opacity factor, denoted by $\alpha$, is computed by multiplying $\gamma$ with the contribution of the 2D covariance, calculated from $\Sigma'$ and the pixel coordinate in image space. The covariance matrix $\Sigma$ is parameterized using a unit quaternion $q$ and a 3D scaling vector $v$ to ensure a meaningful interpretation during optimization.

\textbf{SMPL-X parameterization}  \cite{SMPLX2019} is an extension of the original SMPL body model \cite{SMPL2015} with face and hand, designed to capture more details. detailed and expressive human deformations. \textbf{SMPL-X} expands the joint set of \textbf{SMPL}, including those for the face, fingers, and toes. This allows for a more accurate representation of intricate body movements. \textbf{SMPL-X} is defined by a function $M(\beta, \theta, \psi) : \mathbb{R}^{|\beta| \times |\theta| \times |\psi|} \rightarrow \mathbb{R}^{3N}$, parametrized by the pose $\theta \in \mathbb{R}^{3K}$ (where $K$ denotes the number of body joints), face and hands shape $\beta \in \mathbb{R}^{|\beta|}$ and facial expression $\psi \in \mathbb{R}^{|\psi|}$. To be specific:
\[
M(\beta, \theta, \psi) = W(T_p(\beta, \theta, \psi), J(\beta), W),
\]
where $T_p$ is the human body mesh in the canonical pose, $J$ is the pre-trained regression matrix, $W$ is the pose transformation operation, and $W$ is the predetermined skin blending weight. For more details refer to \cite{SMPLX2019}.

% \subsection{2D animation comparison}
% \label{subsection:2d_anim_compare}

% \input{Figures/2d_animation_comparison}

% \huien{

% Figure \ref{figure:2d_animation_comparison} compares our reconstruction and reposing to 2D animation methods that takes a single frame as input. 
% 3D Reconstruction and reposing has better preservation of body shape and fine-grained details such as face and clothing. Compared to Animate-Anyone and Magic-Animate, DCH is able to to model fine-grained body parts such as hand and faces more accurately. Compared to CHAMP, the reposed results are more consistent. More importantly, the disentanglement allows direct manipulation of the Clothing Gaussians.
% }

\subsection{Training details of animation pipeline}
\label{subsection:anim_implementation}

To optimize the deformation field given the video from the reference view, Mean Square Error (MSE) is used to minimize the distance between the rendered image and video frame at each timestep:
\begin{equation}
\mathcal{L}_{Ref} = \frac{1}{T} \sum_{t=1}^{T} \| f(\phi(S', t), \mathbf{O}_{Ref}) - \mathbf{I}_{Ref}^{\tau} \|_2^2,
\end{equation}
where ${I}_{Ref}^{\tau}$ is the $\tau$-th frame in the video. ${O}_{Ref}$ is the reference view point and $f$ is the rendering function. To propagate the motion from the reference view to the whole 3D model, we leverage  Zero-1-to-3-XL \cite{objaverseXL} to predict the deformation of the unseen part. Although image diffusion models only perform per-frame prediction, the temporal consistency can be mostly preserved since the color and opacity of the static 3D GS are fixed. Similar to the training practice in DreamGaussian4D, multiple views are sampled for each time step:
\begin{equation}
\nabla_{\phi} \mathcal{L}_{SDS} = \mathbb{E}_{t,\tau,\epsilon,o} \left[ (\epsilon_{\theta} ( \tilde{I}; t, \mathbf{I}^{\tau}_{Ref} , o) - \epsilon) \frac{\partial \mathcal{I}}{\partial \phi} \right] 
\end{equation}
\vspace{-5pt}
\begin{equation}
\tilde{I} = f(\phi(S', \tau), o), 
\end{equation}
where $\epsilon$ is a random noise, $\epsilon_{\theta}$ is the noise predictor of a 3D-aware image diffusion model, and $o$ is a random viewpoint.

\subsection{Training details of Identity Encoding loss}
\label{subsection:id_implementation}

\textit{\underline{Grouping via rendering}}. To optimize the introduced Identity Encoding of each Gaussian, we render these encoded identity vectors into 2D images in a differentiable manner following \cite{Ye2023gaussian_grouping}. We take the differentiable 3D Gaussian renderer from \cite{kerbl3Dgaussians} and treat the rendering process similar to the color (SH coefficients) optimization in \cite{kerbl3Dgaussians}. 3D Gaussian splatting adopts neural point-based $\alpha'$-rendering \cite{KPLD21,kopanas2022neural}, where the influence weight $\alpha'$ can be evaluated in 2D for each pixel and each Gaussian. Following  \cite{kerbl3Dgaussians}, the influence of all Gaussians on a single pixel location are computed by sorting the Gaussians in the depth order and blending $N$ ordered points overlapping the pixels:
\begin{equation}
E_{id} = \sum_{i \in \mathcal{N}} e_i \alpha_i \prod_{j=1}^{i-1} (1 - \alpha'_j)
\end{equation}
where the final rendered 2D mask identity feature $E_{id}$ for each pixel is the sum over the Identity Encoding $e_{i}$ of length 15 for each Gaussian, weighted by the Gaussian’s influence factor $\alpha'_i$  on that pixel. We compute $\alpha'_i$ by measuring a 2D Gaussian with covariance $\Sigma2D$ multiplied by a learned per-point opacity $\alpha_i$:
\begin{equation}
\Sigma2D = JW\Sigma2D^{3D}W^{T}J^{T} 
\end{equation}
where $\Sigma3D$ is the 3D covariance matrix, $\Sigma2D$ is the splatted 2D version, J is the Jacobian of the affine approximation of the 3D-2D projection, and W is the world-to-camera transformation matrix.

An unsupervised 3D regularization loss is applied to regularize the learning of Identity Encoding $e_{i}$. This loss enforces the Identity Encodings of the top $k$-nearest 3D Gaussians to be close in their feature distance and encourages 3D spatial consistency. We denote $F$ as the softmax operation, and formalize the KL divergence loss with $m$ sampling points as:
\begin{equation}
\mathcal{L}_{3d} = \frac{1}{m} \sum_{j=1}^{m} D_{KL}(P||Q) = \frac{1}{mk} \sum_{j=1}^{m} \sum_{i=1}^{k} F(e_j) \log \left( \frac{F(e_j)}{F'(e_j)} \right)
\end{equation}
% \vspace{-5pt}
where $P$ contains the sampled Identity Encoding $e$ of a 3D Gaussian, while the set $Q = {e'1, e'2, ..., e'k}$ consists of its $k$-nearest neighbors in the 3D spatial space. The total loss for identity encoding is: 
% \vspace{-5pt}
\begin{equation}
\mathcal{L}_{id} = \mathcal{L}_{2d} + \mathcal{L}_{3d} 
\end{equation}

\subsection{Implementation details}
\label{subsection:training_details}
Experiments were ran on a single 24GB RTX3090 GPU.
%We implement the our reconstruction, disentanglement and editing framework were built upon the open-source repository DreamGaussian \cite{tang2023dreamgaussian} and the animation framework was build on the open-source repository DreamGaussian4D \cite{ren2023dreamgaussian4d}. 
% For driving video generation, we use an open-source implementation of AnimateAnyone \cite{hu2023animateanyone}. 
In our 3D generation process, we performed initial SMPL-X fitting with 3000 iterations in 3 minutes and skin color inpainting on SMPL-X Gaussians for 100 iterations in 30 seconds. Reconstruction and disentanglement optimization required 3000 iterations over 12 minutes. For video reconstruction, SMPL-X fitting aligned 14 frames in 6 minutes for in-the-wild videos. Our 4D-Dress \cite{wang20244ddress} experiments involved 1000 iterations for clothing deformations over 18 minutes, following the methodology described in DreamGaussian4D \cite{ren2023dreamgaussian4d}.

\subsection{Details for Clothing Gaussian Optimization}

\textbf{Embedding on mesh.}
Each 3D clothing Gaussian is embedded on one triangle of the canonical mesh. The embedding directly defines the position of the Gaussians in both canonical and posed space. Other than position, each Gaussian has its own parameters of rotation, scaling, color and opacity. When the mesh is deformed for animation, the embedding provides additional rotation and scaling upon each Gaussian: the pose-dependent rotation is defined by barycentric interpolated per-vertex quaternion while the scaling is defined by the change in the lengths of the embedded triangle. Lastly, the embedding is learned from the Identity Encoding. Using the embedding can significantly accelerate the reposing. 
%reposing is much faster compared to previous reposing methods of finding the nearest neighbours and applying LBS transformation. 
During optimization, the Gaussian parameters and embedding parameters are updated simultaneously.

% positions % 
Given the vertices of a triangle, we define the mean position \( \mathbf{O} \) of the vertices as the origin of the local coordinate system. The local coordinate system for each triangle includes orthogonal basis vectors (x-axis, y-axis) and the normal vector. The x- and y-axis are calculated from normalized edges of the triangle while the normal vector (z-axis) is obtained as the cross product of the edges, thus defining the orthogonal direction to the plane of the triangle. We define the position of a Gaussian (the mean \( \mu \)) by an offset vector \( \mathbf{v} \) from the local origin \( \mathbf{O} \). The displacement vector \( \mathbf{v} \) in local coordinates is applied as follows:
\[
\mathbf{v} = \alpha \mathbf{x\_axis} + \beta \mathbf{y\_axis} + \gamma \mathbf{normal}
\]
where \( \alpha, \beta, \) and \( \gamma \) are the components of the displacement vector along the respective axes. 

The global position \( \mu \) of the Gaussian after applying the displacement, is then calculated by:
\[
\mathbf{\mu} = \mathbf{O} + \mathbf{v}
\]
Unlike SplattingAvatar \cite{SplattingAvatar:CVPR2024}, which defines the position of a Gaussian by a displacement \( \mathbf{d} \) along the interpolated normal vector, a vector position offset \( \mathbf{v} \) from the center of the face \( \mathbf{O} \) is learned. This ensures that Gaussians that are not in the plane of the triangle can still be embedded to the most suitable triangle i.e.  hair Gaussians are tagged to the faces in the head instead of the nearest face used in other reposing methods \cite{SplattingAvatar:CVPR2024,hu2023gauhuman}.

% rotation% 

As proposed by Zielonka et al. \cite{INSTA:CVPR2023}, for the corresponding triangle in the canonical and posed space at frame $t$ we compute the matrix $\mathbf{R}_{cano, pos}$ based on the triangle's tangent, bitangent, and normal to track the triangle rotation from canonical to posed. The rotation matrix is then converted to a quaternion.

We then adopt the rotation of this facet as the Gaussian’s rotation transformation matrix:
% \begin{equation}
% R_i = R_{f_j} = e_{can} \cdot e_{ob}^T,
% \end{equation}
\begin{equation}
r'_i = \text{Rot}(e_{can} \cdot e_{ob}^T, r_i),
\end{equation}
where $r'_i$ is rotated Gaussian rotation, $e_{can}$ and $e_{ob}$ represent the orthonormal bases of the facet in the canonical and observed poses, respectively. These bases are computed from the edge vectors’ normalized cross products. 

% To enhance computational efficiency during training, we precompute the rotation for all faces $R_f$ leveraging the known distribution of SMPL-X poses. To precisely represent the view-dependent colors, the spherical harmonics are rotated together with Gaussians. The spatial descriptions of the original Gaussians $S$ is updated to $S'$ following the reposing.

% and we calculate the per-vertex quaternion $q_v$ by area-weighted average from surrounding neighbor triangles:
% \begin{align*}
%     R_k &= R_{cano}R_{pos}^{-1}, \\
%     q_v &= \frac{\sum_{v \in \mathcal{N}} A_k A_k q_k}{\sum_{v \in \mathcal{N}} A_k},
% \end{align*}
% where $A_k$ are the triangle's area and quaternion respectively. For an embedding $E_i$ with quaternions $\{q_1, q_2, q_3\}$ calculated on the corresponding triangle vertices at frame $t$, the barycentric interpolated rotation $q_{i,t}$ is multiplied to the canonical rotation $q$ of the Gaussian in the canonical space:
% \[
%     \delta q_{i,t} = u q_1 + v q_2 + (1 - u - v) q_3, \quad q_{i,t} = \delta q_{i,t} + q_i.
% \]

% scaling% 

% However, we scale the gaussians by the change in lengths of the triangles. Unlike SplattingAvatar, the lengths are scaled according to the change in length per gaussians instead of area.

In our model, unlike the SplattingAvatar approach which utilizes the area change of the embedded triangle to represent the scaling caused by deformation,
% \[
%     s_{i,t} = \frac{A_{\text{pos}}}{A_{\text{cano}}}.
% \]
we adopt a method where the scaling of Gaussians is based on the change in lengths of the triangles, not just the area. The scaling alterations for each Gaussian are dynamically computed based on individual face transformations, as shown in the algorithm below:
\[
R_k = \frac{S_k}{S_{\text{cano}, k}}
\]

This method allows for more nuanced control over the deformation by scaling according to the change in length of the triangles. This approach, while diverging from traditional area-based scaling methods, provides enhanced flexibility and adaptability in handling complex deformations.

\subsection{Implementation Details}
The 3D generation experiments were conducted using a single 24GB RTX3090 GPU, while the 4D generation experiments utilized a single 48GB RTX6000 GPU. For the 3D generation process, the SMPL-X fitting was performed with 3000 iterations in 3 minutes, followed by skin color inpainting on SMPL-X Gaussians for 100 iterations in 30 seconds. Reconstruction and disentanglement optimization required 3000 iterations, completed in 12 minutes. In video reconstruction, SMPL-X fitting aligned 14 frames in 6 minutes for in-the-wild videos. The 4D-Dress \cite{wang20244ddress} experiments involved 1000 iterations for clothing deformation over 18 minutes.

\clearpage
\subsection{Visual comparisons of 3D Generation and Editing}
\input{Figures/reconstructionv1}

\clearpage
%\begin{landscape}
% \subsection{More visual comparisons of reconstruction and disentanglement}

\input{Figures/reconstruction_appendix}
%\end{landscape}
\clearpage

\subsection{Visual comparison of Animation}

\begin{figure*}[hbt!]
    \centering
    % \subfigure{
    % \vspace{40pt}
    \includegraphics[width=0.95\linewidth ,keepaspectratio]{Figures/Image/anim3.pdf}
    % \rule{10cm}{3cm} % This creates a black rectangle of 6cm x 3cm
    % \rule{10cm}{3cm} % This creates a black rectangle of 6cm x 3cm
    % \vspace{-10pt}
    \caption{\small \textbf{More examples of animation results compared to Dreamgaussian4D.}}
    \label{figure:animation_appendix}
\end{figure*}

% \begin{figure*}[hbt!]
%     \centering
%     % \subfigure{
%     % \includegraphics[width=0.9\textwidth ,keepaspectratio]{Figures/Image/anim.png}
%     \includegraphics[width=0.5\textwidth ,keepaspectratio]{Figures/Image/animation.pdf}
%     \vspace{-10pt}
%     \caption{\small \textbf{Example of animation results compared to Dreamgaussian4D.}}
%     \label{figure:animation}
% \end{figure*}

\begin{wrapfigure}{r}
{0.5\textwidth} 
    %\vspace{-30pt}
    \centering
    \includegraphics[width=0.5\textwidth ,keepaspectratio]{Figures/Image/animation.pdf}
    %\vspace{20pt}    
    \caption{\small \textbf{Examples of animation results compared to Dreamgaussian4D.}}
    \label{figure:animation}
\end{wrapfigure} 
When employing DreamGaussian4D's reconstruction model as initialisation, the resulting Gaussian reconstructions tend to exhibit degraded fidelity in facial regions, limbs, and accessories such as shoes, which often vanish. Utilizing our reconstructed avatar as initialisation improves the quality, but the face and hand details remain suboptimal. Reposing our canonical avatar enables us to align the body and assets accurately with the inferred postures from the source video, yielding high-quality reconstruction of faces, hands, and garments. Despite these improvements, our method does not fully capture aspects not visible in the initial frame, such as the  rear view of the shoes.

\clearpage
\subsection{Visual comparisons to 2D animation methods.}
\input{Figures/2d_animation_comparison}

\subsection{Discussion on failure cases}
\input{Figures/failure_cases}

Despite achieving impressive results, some failures cases still exist, as shown in Figure \ref{figure:failure_cases} in the Appendix. DCH relies on robust and pixel-aligned SMPL-X estimation, which is still an unsolved problem, especially for challenging poses. In Figure \ref{figure:failure_cases}a, it is difficult to correct the pose with keypoints and segmentation mask due to depth ambiguity. DCH occasionally fails for poor visual hull initialization (\ref{figure:failure_cases}b), which is common for difficult poses. Lastly, poor disentanglement is a common problem due to misclassification of clothing category by the segmentation model. This is seen in Figure \ref{figure:failure_cases}c where the arms are wrongly classified under the "top" category.

\subsection{Ablation for initialization}
\input{Figures/ablation_initialisation}

The initialization of clothing Gaussians plays a critical role in high fidelity reconstruction. As illustrated in Figure \ref{figure:ablation_initialisation} in the Appendix, hull-based initialization markedly enhances the accuracy and realism of clothing models compared to random initialization or direct SMPL-X surface initialization. Random initialization tends to produce artifacts as some gaussians do not lie close to the body. For initialization on the SMPL-X surface, the gaussians tend lie close to the body, a problem exacerbated when dealing with complex garments or loosely fitting clothes. These scenarios often lead to the formation of elongated, thin Gaussians as they try to compensate for the large offsets from the body surface, resulting in visual artifacts and blurriness. Conversely, hull-based initialization successfully captures garment details and maintains pose consistency, outperforming the other methods by adhering more closely to the actual geometry of the clothed body.

\clearpage
